# Supplementary material for: Tensor-based Emotion Editing in the StyleGAN Latent Space
Source: arXiv:2205.06102 source file (2022-05-12)
Supplement: Supplementary file 1 [file appendix.tex]

\subsection{Analyzing the Expression Subspace}

\red{
In Fig.~\ref{fig:exprsubspaces} we show a visualization of the expression subspace.
As an initial step we truncated the expression subspace from 25 dimensions to 3D.  
It can be seen that for each emotion, the variation in expression strength form linear trajectories in expression space.  These trajectories are star-shaped and meet at an origin of expression which is shared by all emotion trajectories. We also note that all the expression trajectories  approximately lie in a plane.   
}

% This is neither the neutral nor the mean face, but the ``apathetic''

\begin{figure}[h!]
   \centering
   \includegraphics[width=\linewidth]{figs/expression_apathy.png}
   \caption{Visualization of the expression subspace}
   \label{fig:exprsubspaces}
\end{figure}

\begin{figure}[h!]
   \centering
   \includegraphics[width=\linewidth]{figs/apathy_meanperson.png}
   \includegraphics[width=\linewidth]{figs/apathy_person0.png}
\end{figure}

\subsection{Rank-one vs full rank parameters}

\begin{figure}[h!]
   \centering
   \includegraphics[width=\linewidth]{figs/rankone-vs-fullrank.png}
   \includegraphics[width=\linewidth]{figs/rankone-vs-fullrank-loss.png}
\end{figure}

\section{More}

   % \begin{figure}[h!]
   % \centering
   % \begin{subfigure}[b]{\linewidth}
   % \includegraphics[width=\linewidth]{figs/embed_l1o_original.png}
   % \caption{Original generated images}
   % \end{subfigure}
   
   % \begin{subfigure}[b]{\linewidth}
   % \includegraphics[width=\linewidth]{figs/embed_l1o_rankone.png}
   % \caption{Parameter vectors}
   % \end{subfigure}
   
   % \begin{subfigure}[b]{\linewidth}
   % \includegraphics[width=\linewidth]{figs/embed_l1o_fullrank.png}
   % \caption{Parameter tensor} 
   % \end{subfigure}
   % \end{figure}
   % \begin{figure}[h!]
   % \centering
   % \begin{subfigure}[b]{\linewidth}
   % \includegraphics[width=\linewidth]{figs/embed_generated_original.png}
   % \caption{Original generated images}
   % \end{subfigure}
   
   % \begin{subfigure}[b]{\linewidth}
   % \includegraphics[width=\linewidth]{figs/embed_generated_rankone.png}
   % \caption{Parameter vectors}
   % \end{subfigure}
   
   % \begin{subfigure}[b]{\linewidth}
   % \includegraphics[width=\linewidth]{figs/embed_generated_fullrank.png}
   % \caption{Parameter tensor} 
   % \end{subfigure}
   % \end{figure}
   % \begin{figure}[h!]
   % \centering
   % \begin{subfigure}[b]{\linewidth}
   % \includegraphics[width=\linewidth]{figs/embed_celeb_original.png}
   % \caption{Original generated images}
   % \end{subfigure}
   
   % \begin{subfigure}[b]{\linewidth}
   % \includegraphics[width=\linewidth]{figs/embed_celeb_rankone.png}
   % \caption{Parameter vectors}
   % \end{subfigure}
   
   % \begin{subfigure}[b]{\linewidth}
   % \includegraphics[width=\linewidth]{figs/embed_celeb_fullrank.png}
   % \caption{Parameter tensor} 
   % \end{subfigure}
   % \end{figure}

\subsection{Action units}
\begin{figure}[h!]
\centering
\includegraphics[width=\linewidth]{figs/audiffAnger.png}
\includegraphics[width=\linewidth]{figs/audiffDisgust.png}
\includegraphics[width=\linewidth]{figs/audiffFear.png}
\includegraphics[width=\linewidth]{figs/audiffHappiness.png}
\includegraphics[width=\linewidth]{figs/audiffSadness.png}
\includegraphics[width=\linewidth]{figs/audiffSurprise.png}
\end{figure}

\begin{figure}[h!]
\centering
\includegraphics[width=\linewidth]{figs/mean_expr_plot_Happiness.png}
\includegraphics[width=\linewidth]{figs/mean_expr_plot_Fear.png}
\includegraphics[width=\linewidth]{figs/mean_expr_plot_Anger.png}
\includegraphics[width=\linewidth]{figs/mean_expr_plot_Sadness.png}
\includegraphics[width=\linewidth]{figs/mean_expr_plot_Disgust.png}
\includegraphics[width=\linewidth]{figs/mean_expr_plot_Surprise.png}
\caption{Overview of the effect of applying the direction corresponding to the six prototypical expressions to the BU-3DFE mean face. 
We interpolate in the interval from -3 to 3. Thus the right column shows and edit in the direction of the respective expressions while the left column we have subtracted the expressions from the mean face.}
\label{expression_directions_on_mean_face}
\end{figure}
\subsection{CP decomposition}
\red{[Not yet entirely sure if and how we can use this.]
A tensor can always be decomposed into a sum of rank-one tensors via the Canonical Polyadic (CP) decomposition
\begin{align}
   Q = \sum_r^R \lambda_r \vec{q}_{2,r}\otimes \vec{q}_{3,r} \otimes \vec{q}_{4,r},
\end{align}
where $R$ is the canonical rank of $Q$
}

\subsection{Expression classification}

% \begin{align}
% \vec{q}_5^{\text{frontal} } = 
% \matr{U}_5^\T
% \begin{bmatrix}
%  1/2\\1/2
% \end{bmatrix}
% -\hat{\vec{q}}_5
% \end{align}
% \subsection{Expression Neutralization}
% \subsection{Compressing the latent space}

% \begin{align}
% \tilde{C}_{ijkl} = (S\times_1 \tilde{\matr{U}}_1)_{ijkl}
% \end{align}
% \subsection{Variations}
% For the full model the use the 5 order tensor 
% \begin{align}
%    \hat{w}_i = \bar{w}_i  + C_{ijk\tilde{l}m} Q_{jk\tilde{l}m}
% \end{align}

%%%%%%%%%%%%%%%%% BIN %%%%%%%%%%%%%%%%%%%%%%%%%%

%%%%%%%%%%%%%%%%%%%%%

% Suppose a facial expression dataset contains data points where each of the $E$ emotions are performed with $I$ different levels of intensity. 
% We can then organize the data into a fifth order tensor $\tensor{T}{} \in\mathbb{R}^{D\times P\times E \times I \times R}$ where the $P$ persons perform $E$ expressions with $I$ intensities from $R$ rotations. 
% The corresponding HOSVD of the mean-centered data tensor is
% \begin{align}
% \tensor{T}{} - \bar{\tensor{T}{}} 
% = \tensor{S}{} 
% \times_1 \matr{U}_1 \times_2 \matr{U}_2 \times_3 \matr{U}_3\times_4 \matr{U}_4\times_5 \matr{U}_5
% \end{align}
% % In BU3D-FE each person performs each expression with 4 levels of intensity. 
% % If we discard the neutral expressions

%%%%%%%%%%%%%%%%%%%%

%%%%%%%%%%%%%%%%%%%

\subsection{Multilinear models for faces and expressions}
\red{
%    % Multilinear models in the literature
% 
In the literature, a wide collection of \emph{multilinear} methods have been proposed to model and analyze faces and expressions.  
Early, PCA or dictionary-based 3D Morphable Models (3DMM) \cite{Blanz1999MorphableModel,Ferrari2017Dictionary3DMM} capture the variation in shape and texture of neutral 3D faces. 
% Recently 3DMMs have also been used to make semantic edits to images generated by StyleGAN \cite{Tewari2020Stylerig}.
% More recently, factorization methods, based on higher-order data representations, were introduced with the benefit of better disentanglement of dimensions, such as person-specific shape and expression, when compared to
% matrix methods \cite{tensorface, Vlasic2005}. 
These models were built on the Higher-Order Singular Value Decomposition (HOSVD) to factorize the data, and have successfully been used to model faces, their 3D reconstruction, as well as in transferring expressions \cite{Brunton2014MultilinearWavelets,Chen2014FaceWarehouse}. 
% Moreover, in \cite{apathy,grasshof2020} a HOSVD tensor model was constructed from the Binghamton 3D facial expression database (BU-3DFE) \cite{bu3dfe}, which revealed a practically planar expression subspace, in which the six basic emotions form one-dimensional affine subspaces \cite{apathy}. 
% These six lines intersect in a common vertex, the origin of expressions, which surprisingly does not represent the neutral face, but an extrapolated expression referred to as \emph{apathetic}. 
% is a generalization of the matrix SVD to higher-order tensors.
% \cite{lauth2000,Yano2008,apathy,Multilinearsubspace,tensorface,tensorReview}. 
}
